# Supplementary material for: MalCL: Leveraging GAN-Based Generative Replay to Combat Catastrophic Forgetting in Malware Classification
Source: arXiv:2501.01110 source file (2025-01-02)
Supplement: Supplementary file 1 [file 8_Appendix.tex]

% \section{Number of Classes of selected samples.}

% \begin{figure}[!ht]
%     \centering
%     \begin{subfigure}[b]{0.475\linewidth}
%         \includegraphics[width=\linewidth]{figures/class_count_BCE.png}
%         \caption{when applying BCE.}
%         \label{fig:class_cnt_BCE}
%     \end{subfigure}
%     \hfill
%     \begin{subfigure}[b]{0.475\linewidth}
%         \includegraphics[width=\linewidth]{figures/class_count_FML.png}
%         \caption{when applying FML.}
%         \label{fig:class_cnt_FML}
%     \end{subfigure}

%     \caption{Classes of selected samples on each tasks.}
%     \label{fig:overall}
%     \vskip -0.3cm
% \end{figure}


% To verify whether the Global Selection scheme(Per-Batch Mean Logit Vector) performs effectively, we checked the number of classes of Synthetic samples that the scheme selects, per each task. The middle points represent the mean value from 6 iterations, and the vertical lines are based on the standard deviation from 6 iterations. The total class number of first task is 50, but this selection scheme selects the samples from less than 10 classes. The similar results are for the other tasks. The number of total classes increases as the task goed on, but the number of selected classes is less than 10.

% \section{Environment for the experiments}

% The following table describes the software and hardware environment used for the experiments:

% \begin{table}[h!]
% \centering
% \begin{tabular}{ll}
% \toprule
% \textbf{Component}          & \textbf{Version/Details} \\
% \midrule
% PyTorch                     & 11.8                     \\
% Conda                       & 22.9.0                   \\
% Python                      & 3.12.5                   \\
% NVIDIA GPU                  & RTX A6000                \\
% CIDA                        & 11.4                     \\
% \bottomrule
% \end{tabular}
% \caption{Software and hardware environment used for the experiments.}
% \label{tab:environment}
% \end{table}


% \section{Evaluating MalCL using AZ-Class dataset.}
% \label{app:az-class}
% \begin{figure}[!t]
%    \centering
%     \includegraphics[width=0.7\linewidth]{figures/07.png}
%     \caption{MalCL Performance on the EMBER and AZ-Class datasets using FML and L1-norm to Mean Logits.}
%     \label{fig:dataset}
%     \vskip -0.3cm
% \end{figure}

% To demonstrate that MalCL can be extended to detect Android malware families, we further evaluated MalCL using the AndroZoo dataset (AZ-Class). As shown in Figure~\ref{fig:dataset}, MalCL exhibits better detection accuracy compared to its performance with Windows malware families in the Ember dataset. Overall, MalCL effectively detects both malware datasets amidst the continual emergence of new malware families.
